# Supplementary material for: Audio-Visual Speech Codecs: Rethinking Audio-Visual Speech Enhancement by Re-Synthesis
Source: arXiv:2203.17263 source file (2022-03-31)
Supplement: Supplementary file 1 [file appendix_dump.tex]

\begin{table}[t]
\footnotesize
\centering
\begin{tabular}{|c|c|}
\hline
\textbf{Disentangled Latent Space} & \textbf{Mel-Spectrogram Error} \\ \hline
O                                  & 0.0051424387                   \\ \hline
X                                  & 0.0049852496                   \\ \hline
\end{tabular}
\caption{}
\label{table:disentangling}
\end{table}

%\textbf{Evaluation of Speaker/Content Disentanglement.} We hypothesize that disentangling the speech content from speaker identity better enables the auto-regressive model to generalize across speakers. Table \ref{table:disentangling} supports our hypothesis, demonstrating that our model outperforms a baseline model that does not employ a disentangling strategy for learning speech codes. 

\begin{table*}[t]
\footnotesize
\centering
\begin{tabular}{|l|l|l|l|l|l|l|l|l|l|}
\hline
\textbf{Model}     & \textbf{PESQ}    & \textbf{STOI}    & \textbf{SRMR}     & \textbf{FW-SSNR} & \textbf{MCD}     & \textbf{CSIG}    & \textbf{CBAK}    & \textbf{COVL}    & \textbf{Mel-Spec-Dist} \\ \hline
\multicolumn{10}{|c|}{\textbf{Speaker: J}}                                                                                                                                                           \\ \hline
Masking            & 1.14776          & 0.46980          & 6.62140           & 4.24360          & 6.20473          & 1.99496          & 1.54530          & 1.45248          & 0.01438                \\ \hline
Demucs             & 1.15890          & 0.47643          & 6.02307           & 4.42417          & 5.19233          & 2.40547          & 1.62800          & 1.68634          & 0.01272                \\ \hline
AV Masking         & 1.23358          & 0.56699          & 6.74389           & 5.51005          & 4.98967          & 2.47190          & 1.70990          & 1.75237          & 0.00878                \\ \hline
AV Encoder Decoder & 1.29261          & 0.59604          & 4.85026           & 1.22292          & 4.83129          & 1.01206          & 1.03762          & 1.00146          & 0.00521                \\ \hline
Ours               & \textbf{1.38439} & \textbf{0.65053} & \textbf{9.18364}  & \textbf{7.40862} & \textbf{3.45263} & \textbf{3.07892} & \textbf{1.83733} & \textbf{2.17670} & \textbf{0.00458}       \\ \hline
\multicolumn{10}{|c|}{\textbf{Speaker: BYJ}}                                                                                                                                                         \\ \hline
Masking            &                  &                  &                   &                  &                  &                  &                  &                  &                        \\ \hline
Demucs             & 1.34451          & 0.63211          & 6.12786           & 6.78094          & 4.81492          & 2.70659          & \textbf{1.76722} & 1.95598          & 0.00861                \\ \hline
AV Masking         & 1.28044          & 0.62031          & 6.58130           & 6.47263          & 5.38031          & 2.45899          & 1.67935          & 1.77735          & 0.00985                \\ \hline
AV Encoder Decoder & \textbf{1.37338} & 0.65744          & 4.37330           & 4.38120          & 4.93982          & 1.51396          & 1.30424          & 1.19959          & \textbf{0.00659}       \\ \hline
Ours               & 1.32471          & \textbf{0.67216} & \textbf{6.75246}  & \textbf{7.23640} & \textbf{4.17850} & \textbf{2.76360} & 1.70470          & \textbf{1.95908} & 0.00667                \\ \hline
\multicolumn{10}{|c|}{\textbf{Speaker: CSM}}                                                                                                                                                         \\ \hline
Masking            &                  &                  &                   &                  &                  &                  &                  &                  &                        \\ \hline
Demucs             & \textbf{1.23990} & \textbf{0.55875} & 3.52594           & \textbf{7.44483} & 4.28846          & \textbf{2.83183} & \textbf{1.82996} & \textbf{1.98445} & 0.00723                \\ \hline
AV Masking         & 1.14456          & 0.48871          & \textbf{4.12707}  & 5.01426          & 5.86391          & 2.26566          & 1.63593          & 1.61019          & 0.01256                \\ \hline
AV Encoder Decoder & 1.19823          & 0.51744          & 2.59900           & 0.10221          & 5.26292          & 1.01990          & 1.09156          & 1.00035          & 0.00713                \\ \hline
Ours               & 1.12518          & 0.53337          & 2.60491           & 5.62245          & \textbf{4.21757} & 2.60495          & 1.60976          & 1.77019          & \textbf{0.00702}       \\ \hline
\multicolumn{10}{|c|}{\textbf{Speaker: QEU}}                                                                                                                                                         \\ \hline
Masking            &                  &                  &                   &                  &                  &                  &                  &                  &                        \\ \hline
Demucs             & \textbf{1.39001} & \textbf{0.64591} & 8.12165           & \textbf{7.18049} & 4.81467          & \textbf{2.74161} & \textbf{1.80447} & \textbf{2.00840} & 0.00852                \\ \hline
AV Masking         & 1.21155          & 0.58022          & 7.65505           & 5.60138          & 6.09288          & 2.14685          & 1.59335          & 1.57363          & 0.01249                \\ \hline
AV Encoder Decoder & 1.23609          & 0.59813          & 3.76482           & 2.56998          & 5.31641          & 1.08949          & 1.06554          & 1.01088          & \textbf{0.00749}       \\ \hline
Ours               & 1.26153          & 0.63197          & \textbf{9.34116}  & 6.62152          & \textbf{4.54752} & 2.60108          & 1.64525          & 1.84415          & 0.00779                \\ \hline
\multicolumn{10}{|c|}{\textbf{Speaker: XJO}}                                                                                                                                                         \\ \hline
Masking            & \textbf{}        & \textbf{}        & \textbf{}         & \textbf{}        & \textbf{}        & \textbf{}        & \textbf{}        & \textbf{}        & \textbf{}              \\ \hline
Demucs             & \textbf{1.37143} & 0.68045          & 7.45208           & 7.60437          & 4.28929          & 2.87763          & \textbf{1.84489} & \textbf{2.07367} & 0.00708                \\ \hline
AV Masking         & 1.23933          & 0.61175          & 8.06822           & 5.79868          & 5.94382          & 2.23005          & 1.64048          & 1.63362          & 0.01166                \\ \hline
AV Encoder Decoder & 1.33900          & 0.64655          & 4.33222           & 3.22839          & 4.92964          & 1.11840          & 1.10041          & 1.02754          & 0.00649                \\ \hline
Ours               & 1.36242          & \textbf{0.68906} & \textbf{10.48990} & \textbf{7.60150} & \textbf{3.91303} & \textbf{2.91341} & 1.79515          & 2.07187          & \textbf{0.00567}       \\ \hline
\end{tabular}
\caption{}
\end{table*}

\begin{table*}[t]
\footnotesize
\centering
\begin{tabular}{|l|l|l|l|l|l|l|l|l|l|}
\hline
\textbf{Model}     & \textbf{PESQ}              & \textbf{STOI}    & \textbf{SRMR}     & \textbf{FW-SSNR}  & \textbf{MCD}     & \textbf{CSIG}    & \textbf{CBAK}    & \textbf{COVL}    & \textbf{Mel-Spec-Dist} \\ \hline
\multicolumn{10}{|c|}{\textbf{Speaker: Chemistry Lectures}}                                                                                                                                                     \\ \hline
Masking            & 1.22562 / 1.54674          & 0.66807          & 7.39356           & 5.81697           & 6.86629          & 1.95135          & 1.45153          & 1.49565          & 0.01840                \\ \hline
Demucs             & 1.30798 / 1.68731          & 0.73130          & 6.98558           & 6.99200           & 5.34305          & 2.54446          & 1.65219          & 1.85763          & 0.01610                \\ \hline
AV Masking         & 1.31894 / 1.70456          & 0.71744          & 7.10656           & 7.18660           & 5.59763          & 2.47591          & 1.59114          & 1.81000          & 0.01160                \\ \hline
AV Encoder Decoder & 1.48498 / 1.87732          & 0.75118          & 5.96917           & 7.29518           & 4.41298          & 2.69499          & 1.72553          & 1.97488          & 0.00568                \\ \hline
Ours               & \textbf{1.50267 / 1.95634} & \textbf{0.80746} & \textbf{10.07557} & \textbf{9.24735}  & \textbf{3.72522} & \textbf{3.13018} & \textbf{1.88548} & \textbf{2.26355} & \textbf{0.00486}       \\ \hline
\multicolumn{10}{|c|}{\textbf{Speaker: Chess Lectures}}                                                                                                                                                         \\ \hline
Masking            & 1.25125 / 1.67366          & 0.69380          & 3.98470           & 7.73761           & 6.37667          & 2.33859          & 1.64880          & 1.74772          & 0.01204                \\ \hline
Demucs             & \textbf{1.52612 / 2.04458} & \textbf{0.82022} & 3.15778           & \textbf{10.18910} & \textbf{4.06913} & \textbf{3.17828} & \textbf{1.98597} & \textbf{2.33529} & 0.00625                \\ \hline
AV Masking         & 1.42596 / 1.92076          & 0.75641          & \textbf{4.05624}  & 9.12770           & 5.06899          & 2.86791          & 1.83274          & 2.11292          & 0.00703                \\ \hline
AV Encoder Decoder & 1.36009 / 1.75666          & 0.70607          & 3.48531           & 7.46564           & 4.87580          & 2.53313          & 1.64341          & 1.82929          & 0.00521                \\ \hline
Ours               & 1.39311 / 1.83390          & 0.77441          & 2.90414           & 9.54627           & 4.30888          & 3.00602          & 1.86712          & 2.16222          & \textbf{0.00467}       \\ \hline
\multicolumn{10}{|c|}{\textbf{Speaker: Deep Learning Lectures}}                                                                                                                                                 \\ \hline
Masking            & 1.33614 / 1.67006          & 0.51759          & 8.54157           & 6.37243           & 6.28671          & 2.20022          & 1.53087          & 1.65784          & 0.01401                \\ \hline
Demucs             & 1.33554 / 1.63653          & 0.56621          & 8.95677           & 7.04893           & 4.75619          & 2.63600          & 1.57814          & 1.89484          & 0.01236                \\ \hline
AV Masking         & \textbf{1.53896 / 1.93040} & 0.65148          & 9.75917           & 8.10135           & 5.09919          & 2.75767          & 1.72756          & 2.06919          & 0.00975                \\ \hline
AV Encoder Decoder & 1.47203 / 1.77278          & 0.62747          & 6.14487           & 7.03200           & 4.62598          & 2.35859          & 1.43507          & 1.72117          & 0.00646                \\ \hline
Ours               & 1.53851 / 1.87068          & \textbf{0.70466} & \textbf{11.52928} & \textbf{8.68379}  & \textbf{4.30770} & \textbf{2.94586} & \textbf{1.81646} & \textbf{2.17064} & \textbf{0.00585}       \\ \hline
\multicolumn{10}{|c|}{\textbf{Speaker: Ethical Hacking Lectures}}                                                                                                                                               \\ \hline
Masking            & 1.34706 / 1.78550          & 0.53011          & 7.17107           & 5.83375           & 6.31656          & 2.18427          & 1.50304          & 1.64730          & 0.01316                \\ \hline
Demucs             & 1.32090 / 1.71762          & 0.61269          & 9.10952           & 7.36614           & 4.38185          & 2.71547          & 1.75968          & 1.94718          & 0.00924                \\ \hline
AV Masking         & 1.38733 / 1.86672          & 0.65502          & 9.40703           & 7.53899           & 4.88785          & 2.69967          & 1.65148          & 1.95516          & 0.00841                \\ \hline
AV Encoder Decoder & 1.38957 / 1.82827          & 0.62951          & 7.10116           & 6.30792           & 4.27300          & 2.48803          & 1.57086          & 1.77838          & 0.00561                \\ \hline
Ours               & \textbf{1.49106 / 1.96994} & \textbf{0.72235} & \textbf{13.10427} & \textbf{8.66450}  & \textbf{3.59204} & \textbf{3.07259} & \textbf{1.83176} & \textbf{2.21067} & \textbf{0.00475}       \\ \hline
\multicolumn{10}{|c|}{\textbf{Speaker: Hardware Security Lectures}}                                                                                                                                             \\ \hline
Masking            & 1.34011 / 1.69624          & 0.54093          & 10.27053          & 5.64497           & 6.57306          & 2.02189          & 1.51301          & 1.56180          & 0.01400                \\ \hline
Demucs             & 1.42386 / 1.78936          & 0.63114          & 11.48057          & 6.62148           & 5.06925          & 2.62721          & 1.70412          & 1.93704          & 0.01062                \\ \hline
AV Masking         & \textbf{1.52059 / 1.92807} & 0.66431          & 11.04458          & 7.41151           & 5.18016          & 2.69850          & 1.70052          & 2.02196          & 0.00950                \\ \hline
AV Encoder Decoder & 1.37870 / 1.68562          & 0.58929          & 5.08994           & 6.35713           & 5.02736          & 2.43028          & 1.50795          & 1.76483          & 0.00800                \\ \hline
Ours               & 1.48658 / 1.83152          & \textbf{0.68975} & \textbf{12.87511} & \textbf{7.86225}  & \textbf{4.42849} & \textbf{2.87844} & \textbf{1.70350} & \textbf{2.10454} & \textbf{0.00747}       \\ \hline
\end{tabular}
\caption{}
\end{table*}

\begin{table*}[]
\footnotesize
\begin{tabular}{lllll}
Model                                                                            & Speaker S1   & Speaker S3   & Speaker S11  & Speaker S15  \\
Single Speaker                                                                   & 0.0050910308 & 0.0079405317 & 0.0074597462 & 0.0078080879 \\
\begin{tabular}[c]{@{}l@{}}Multi Speaker, \\    \\ Not Finetuned\end{tabular}    & 0.0065759142 & 0.0090927205 & 0.0096039879 & 0.0159421251 \\
%\begin{tabular}[c]{@{}l@{}}Multi Speaker, \\    \\ Finetuned (0.05)\end{tabular} & 0.0066588236 & 0.0090580166 & 0.0095705614 & 0.0161205846 \\
\begin{tabular}[c]{@{}l@{}}Multi Speaker, \\    \\ Finetuned (0.1)\end{tabular}  & 0.0048062729 & 0.0068266065 & 0.0062532304 & 0.0068085396 \\
\begin{tabular}[c]{@{}l@{}}Multi Speaker, \\    \\ Finetuned (0.25)\end{tabular} & 0.0045704261 & 0.0061953527 & 0.0058948261 & 0.0065535355 \\
\begin{tabular}[c]{@{}l@{}}Multi Speaker, \\    \\ Finetuned (0.5)\end{tabular}  & 0.0044332177 & 0.0059520817 & 0.0056976204 & 0.0062116304 \\
\begin{tabular}[c]{@{}l@{}}Multi Speaker, \\    \\ Finetuned (1.0)\end{tabular}  & 0.0042566591 & 0.0056138235 & 0.0055347989 & 0.0059580329
\end{tabular}
\end{table*}

\begin{table}[]
\begin{tabular}{|l|l|}
\hline
SNR                                                                                      & Mel-Spec MSE \\ \hline
\begin{tabular}[c]{@{}l@{}}Autoencoder Reconstruction\\    \\ (Lower Bound)\end{tabular} & 0.0009470281 \\ \hline
0-10                                                                                     & 0.0029131919 \\ \hline
10-20                                                                                    & 0.0020808217 \\ \hline
20-30                                                                                    & 0.0015940420 \\ \hline
30-40                                                                                    & 0.0012731550 \\ \hline
\end{tabular}
\end{table}

\begin{table*}[t]
\footnotesize
\centering
    \begin{tabular}{|l|l|l|l|l|l||l|l|l|l|}
    \hline
    \textbf{Model}      & \textbf{PESQ}     & \textbf{STOI}     & \textbf{FW-SSNR}      & \textbf{MCD}      & \textbf{Mel-Spec-Dist}        & \textbf{SRMR}     & \textbf{CSIG}     & \textbf{CBAK}     & \textbf{COVL}     \\ \hline
    \multicolumn{10}{|c|}{\textbf{Speaker 1 (Female)}}      \\ \hline
    Masking     & 1.14776       & 0.46980       & 4.24360       & 6.20473       & 0.01438       & 6.62140       & 1.99496       & 1.54530       & 1.45248       \\ \hline
    Demucs      & 1.15890       & 0.47643       & 4.42417       & 5.19233       & 0.01272       & 6.02307       & 2.40547       & 1.62800       & 1.68634       \\ \hline
    AV Masking      & 1.23358       & 0.56699       & 5.51005       & 4.98967       & 0.00878       & 6.74389       & 2.47190       & 1.70990     & 1.75237       \\ \hline
    AV Encoder Decoder      & 1.29261       & 0.59604       & 1.22292       & 4.83129       & 0.00521       & 4.85026       & 1.01206       & 1.03762       & 1.00146       \\ \hline
    Ours        & \textbf{1.38439}      & \textbf{0.65053}      & \textbf{7.40862}      & \textbf{3.45263}      & \textbf{0.00458}      & \textbf{9.18364}        & \textbf{3.07892}      & \textbf{1.83733}      & \textbf{2.17670}      \\ \hline
    \multicolumn{10}{|c|}{\textbf{Speaker 2 (Male)}}        \\ \hline
    Masking     &       &       &       &       &       &       &       &       &       \\ \hline
    Demucs      & 1.34451       & 0.63211       & 6.78094       & 4.81492       & 0.00861       & 6.12786       & 2.70659       & \textbf{1.76722}        & 1.95598       \\ \hline
    AV Masking      & 1.28044       & 0.62031       & 6.47263       & 5.38031       & 0.00985       & 6.58130       & 2.45899       & 1.67935     & 1.77735       \\ \hline
    AV Encoder Decoder      & \textbf{1.37338}      & 0.65744        & 4.38120      & 4.93982       & \textbf{0.00659}      & 4.37330       & 1.51396       & 1.30424       & 1.19959       \\ \hline
    Ours        & 1.32471       & \textbf{0.67216}      & \textbf{7.23640}      & \textbf{4.17850}      & 0.00667       & \textbf{6.75246}      & \textbf{2.76360}      & 1.70470       & \textbf{1.95908}      \\ \hline
    \end{tabular}
\caption{\textbf{Quantitative Evaluation of Audio-Visual Speech Separation and Enhancement on the Facestar dataset.} Our approach consistently outperforms the baselines. For PESQ, STOI, SRMR, FW-SSNR, CSIG, CBAK, and COVL, higher is better. For MCD and Mel-Spec-Dist, lower is better. See text for details.\DM{Merge speakers 1 and 2}}
\label{table:facestarj}
\end{table*}

\begin{table}[]
\centering
\footnotesize
\begin{tabular}{|c|c|c|}
\hline
\rowcolor[gray]{0.8}
\multicolumn{1}{|l|}{} & \textbf{\begin{tabular}[c]{@{}c@{}}Decoded from\\ GT Mel-Spectrograms\end{tabular}} & \textbf{Ground Truth} \\ \hline
\rowcolor[gray]{0.99}
\textbf{PESQ $\uparrow$} & 2.49504 & 5.0 \\ 
\rowcolor[gray]{0.9}
\textbf{STOI $\uparrow$} & 0.88038 & 1.0 \\ 
\rowcolor[gray]{0.99}
\textbf{MCD $\downarrow$} & 1.68988 & 0.0 \\ 
\rowcolor[gray]{0.9}
\textbf{Mel-Spec-Dist $\downarrow$} & 0.00069 & 0.0 \\ \hline \hline
\rowcolor[gray]{0.99}
\textbf{CSIG $\uparrow$} & 4.26524 & 5.0 \\ 
\rowcolor[gray]{0.9}
\textbf{CBAK $\uparrow$} & 2.53051 & 5.0 \\ 
\rowcolor[gray]{0.99}
\textbf{COVL $\uparrow$} & 3.37861 & 5.0 \\ \hline
\end{tabular}
\caption{\textbf{Objective metrics evaluated on clean synthesized speech.} For PESQ, STOI, CSIG, CBAK, and COVL, higher is better. For MCD and Mel-Spec-Dist, lower is better. See text for details.}
\label{table:decoded_from_melspec}
\end{table}

DATASET TECHNICAL DETAILS 
Video was captured using two synchronized OV2312 1600 x 1300 RGBIr cameras running at 60 fps. A custom camera aggregator sends video streams over USB to PC where they are recorded. Audio was captured using a custom 3D printed microphone array with 7 DPA 4060 pre-polarized condenser microphones. The microphone signals are recorded by an 8 channel RME OctaMic XTC analog to digital converter running at 48kHz. The 8th channel records a shared IRIG timecode signal from a Meinberg syncbox, which is used to synchronize the video and audio subsystems. Note that in this work we use a single camera and a single microphone as inputs of our model.

SNEEZING FIGURE
\begin{figure}
    \centering
    \includegraphics[scale=0.3]{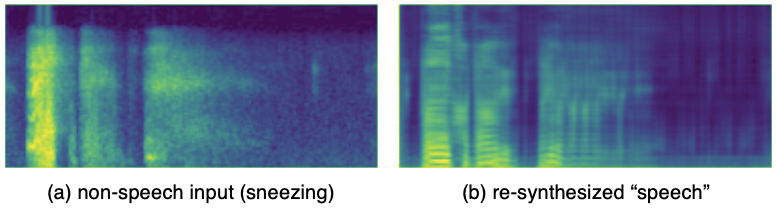}
    \caption{\textbf{Effect of Speech Codebook}. (a) Mel-spectrogram representation of noise. (b) Mel-spectrogram representation of the same noise from (a) after being converted to and reconstructed from speech codes. The reconstructed noise resembles plausible vocal sounds from the target speaker. See supplemental video for examples.}
    \label{fig:codebook_analysis}
\end{figure}

\paragraph{Importance of Speech Codebook.} Our discrete speech codebook, which encodes only sounds from the target speaker, prevents other noise from being propagated through the decoder and synthesized into the output. To demonstrate, we take noise audio clips $N$ and find the sequence of codes that most closely generates this audio, \ie, we optimize:
\begin{equation}
    \min_{\mathbf{Z}} || \mathcal{D}(\mathbf{Z}) – \textbf{melspec}(N) ||_2
\end{equation}
Figure \ref{fig:codebook_analysis} shows an example result of this optimization: a noise clip (Figure \ref{fig:codebook_analysis}(a)) is mapped to a sequence of codes that synthesizes a plausible sound from the target speaker, even though the codes are selected to reproduce the noise.

ATTENTION FIGURE
\begin{figure}
    \centering
    \includegraphics[scale=0.2]{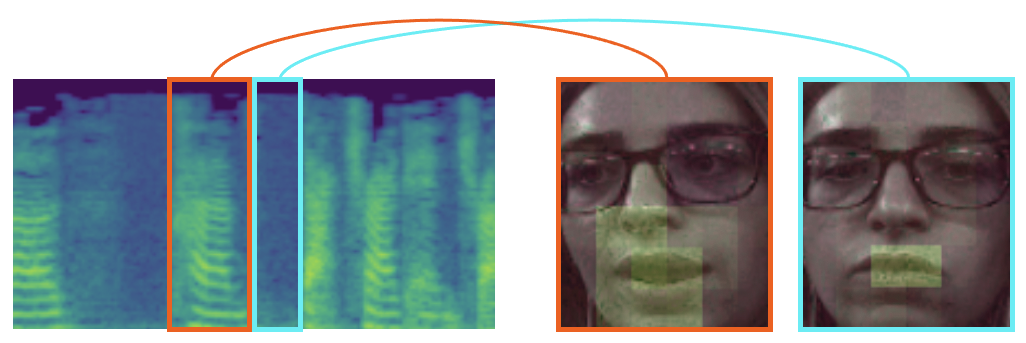}
    \caption{\textbf{Illustration of Visual Attention.} \AR{keep or remove?} Figure shows mel-spectrogram of denoised speech, and images overlaid with heatmaps showing where the visual model attends to.}
    \label{fig:visual_attention}
\end{figure}
